# Supplementary material for: ONER: Online Experience Replay for Incremental Anomaly Detection
Source: arXiv:2412.03907 source file (2025-03-26)
Supplement: Supplementary file 1 [file supplementation.tex]

\clearpage

\setcounter{page}{1}
\maketitlesupplementary
\begin{appendices}

\begin{table*}[tp]
\centering
{\scriptsize
%\begin{tabular}{|c|c|c|c|c|c|c|c|c|c|c|c|c|c|c|}
\begin{tabular}{ccccccccccccccc}
\hline
\textbf{bottle} & \textbf{cable} & \textbf{capsule} & \textbf{carpet} & \textbf{grid} & \textbf{hazelnut} & \textbf{leather} & \textbf{metal\_nut} & \textbf{pill} & \textbf{screw} & \textbf{tile} & \textbf{toothbrush} & \textbf{transistor} & \textbf{wood} & \textbf{zipper} \\
\hline
91.57 & 98.67 & 100 & 90.60 & 75.64 & 79.09 & 50.81 & 99.13 & 98.20 & 100 & 94.02 & 80.95 & 100 & 88.61 &  91.39\\
\hline
\end{tabular}}
\caption{Classification accuracy for each category on the MVTec AD dataset at the task identification stage for UCAD.}
\label{tab:accuracy}
\end{table*}
\begin{table}[!ht]
\centering
{\footnotesize
\begin{tabular}{lcccc}
\toprule
\textbf{Method} & \multicolumn{2}{c}{\textbf{ACC} $\uparrow$} & \multicolumn{2}{c}{\textbf{FM} $\downarrow$} \\
\cmidrule(lr){2-3} \cmidrule(lr){4-5}
 &   \textbf{AUROC} & \textbf{AUPR} & \textbf{AUROC} & \textbf{AUPR} \\
\midrule
% \multicolumn{5}{l}{\textit{Incremental Anomaly Detection Methods}} \\
UCAD & 86.66 & 10.94 & 12.52 & 22.78 \\
Ours & \textbf{99.44} & \textbf{45.43} & \textbf{0.03} & \textbf{1.16}\\
\bottomrule
\end{tabular}}
\caption{Comparison of Pixel-level ACC and FM on the category leather of the MVTec AD dataset after training on the last subset.}
\label{tab:pixel-leather}
\end{table}
\section{Comparison with current sota method: UCAD~\cite{liu2024unsupervised}}
%UCAD utilizes contrastive prompt learning to introduce a continual prompting module that adapts to incremental tasks and facilitates segmentation. 
In the framework of UCAD, contrastive prompt learning is utilized to introduce a continual prompting module that adapts to incremental tasks and facilitates segmentation. 
%Besides, UCAD trains distinct prompts for each task and stores a triplet comprising the prompt, knowledge extracted using a ViT model, and key features stored in a memory bank. 
Besides, UCAD trains distinct prompt for each task and stores a triplet comprising the prompt, knowledge extracted by a ViT, and key features stored in a memory bank. 
%During inference, UCAD employs a two-stage process: it first identifies the task associated with the input image by comparing its features (extracted using a pre-trained ViT) with keys in the memory bank, then applies the corresponding prompt and knowledge to detect anomalies.
During inference, UCAD employs a two-stage process: it first identifies the task associated with the input image by comparing its features with keys in the memory bank, then applies the corresponding prompt and knowledge to detect anomalies.

\begin{figure}[t]
    \centering
    \includegraphics[width=0.9\linewidth]{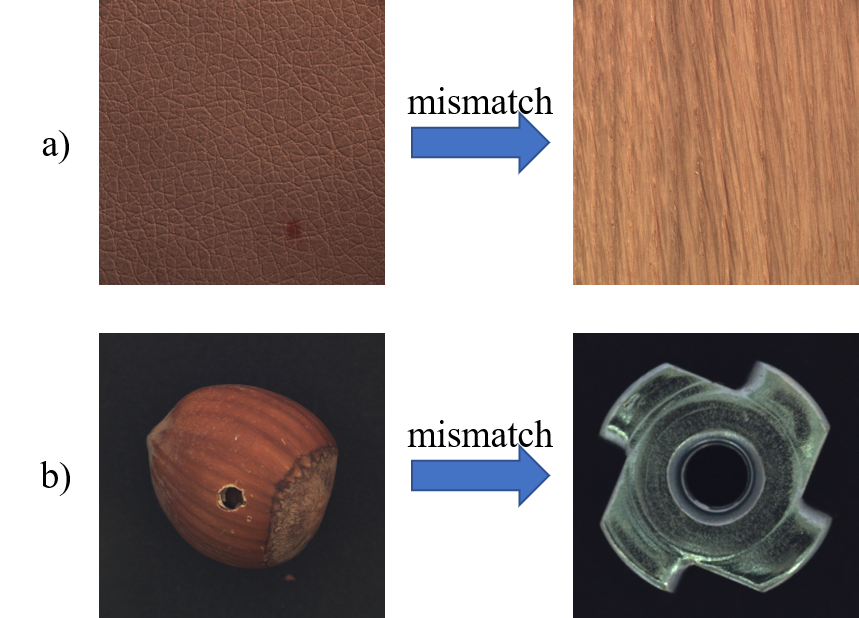}
    \caption{Typical mismatch cases in UCAD. (a) An image from the leather category is mistakenly identified as wood. (b) An image from hazelnut category is mismatched as metal\_nut.}
    \label{fig:mismatch}
\end{figure}
\begin{figure}[t]
    \centering
    \includegraphics[width=0.95\linewidth]{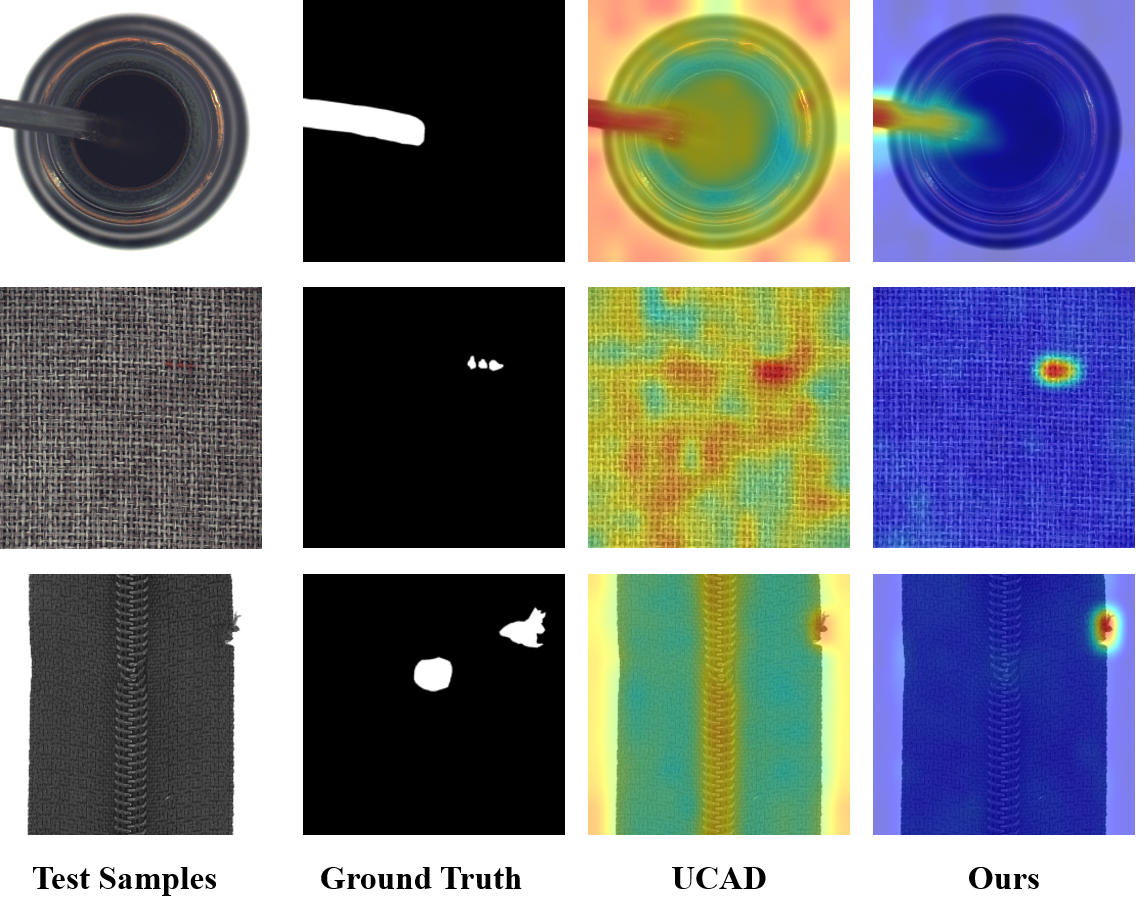}
    \caption{Impact of Task Misidentification on UCAD's Performance.}
    \label{fig:visual2}
\end{figure}
\begin{figure}[t]
\centering
\includegraphics[width=0.46\textwidth]{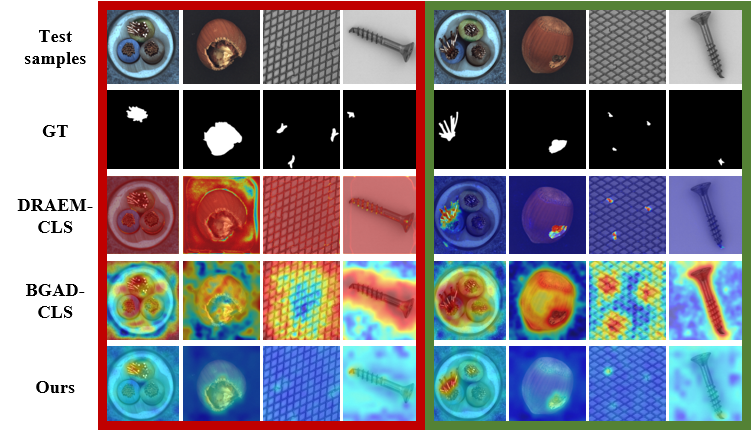} % Reduce the figure size so that it is slightly narrower than the column.
%\caption{Impact of Task Misidentification on Staged Model's Performance.}
\caption{Qualitative evaluation between stage approach and ours. Compared with stage approach which suffers from task misidentification (red), our method is more stable and accurate in anomaly detection. }
\label{fig3}
\end{figure}
%This approach has two major drawbacks. 
UCAD has two major drawbacks. 
% First, it compromises unstable results. 
% Specifically, the task identification of UCAD depends on the ViT which is initially pre-trained on ImageNet. 
% However, a distribution shift exists between ImageNet and real-world images, which can diminish the reliability of classification. 
% As shown in Fig.~\ref{fig:mismatch}, two typical mismatches in UCAD are presented due to task similarity and background similarity, respectively.
% Tab.~\ref{tab:accuracy} displays the classification accuracy across all categories in MVTec AD during the task identification phase of UCAD. 
% Notably, the leather's classification accuracy is significantly low, marked at only 50.81\%.
% Tab.~\ref{tab:pixel-leather} illustrates the performance degradation of UCAD on the leather category, highlighting the unreliability and cumulative task identification errors of UCAD's two-stage method~(shown in Fig.~\ref{fig:visual2}).
% In contrast, our method is task-free and directly detects anomalies from the input image, yielding more stable results.
First, UCAD demonstrates instability in its performance due to its reliance on task identification through feature matching with a pre-trained Vision Transformer (ViT). Since the ViT is trained on ImageNet, a substantial distribution shift exists between ImageNet and real-world industrial test images, rendering the feature-matching-based task identification process unreliable.  As illustrated  in Fig.~\ref{fig:mismatch}, task identification in UCAD is particularly affected by semantic similarities between tasks and the resemblance of foreground and background features across tasks. Tab.~\ref{tab:accuracy} presents the task identification accuracy across all categories in the MVTec AD dataset, highlighting significant challenges. For instance, the accuracy for the leather category is particularly low, at just 50.81\%, which severely impacts it's performance~(shown in Tab.~\ref{tab:pixel-leather}). As illustrated in Fig.~\ref{fig:visual2}, task identification errors often result in incorrect prompt selection, leading to complete detection failures and, consequently, unstable anomaly detection outcomes. In contrast, our end-to-end approach eliminates the need for task identification altogether. By directly detecting anomalies from input images, our method ensures more stable and reliable results, overcoming the limitations observed in UCAD.

\begin{table*}[!ht]
\centering
{\footnotesize
\begin{tabular}{lcccccccc}
\toprule
\multirow{2}{*}{\textbf{Method}} & \multicolumn{4}{c}{\textbf{Pixel-level}} & \multicolumn{4}{c}{\textbf{Image-level}} \\
\cmidrule(lr){2-5} \cmidrule(lr){6-9}
& \multicolumn{2}{c}{\textbf{ACC} $\uparrow$} & \multicolumn{2}{c}{\textbf{FM} $\downarrow$} & \multicolumn{2}{c}{\textbf{ACC} $\uparrow$} & \multicolumn{2}{c}{\textbf{FM} $\downarrow$} \\
\cmidrule(lr){2-3} \cmidrule(lr){4-5} \cmidrule(lr){6-7} \cmidrule(lr){8-9}
& \textbf{AUROC} & \textbf{AUPR} & \textbf{AUROC} & \textbf{AUPR} & \textbf{AUROC} & \textbf{AUPR} & \textbf{AUROC} & \textbf{AUPR} \\
\midrule
% \multicolumn{5}{l}{\textit{Incremental Anomaly Detection Methods}} \\
Baseline + L2P   & \underline{93.56} & \underline{42.66} & \underline{2.09} & \underline{2.14} &  \underline{91.86} & 95.76 & 0.73 &  0.31\\
Baseline + DualPrompt   & 92.79 & 41.32 & 2.83 & 9.63 & 91.81 & \underline{5.77} & 1.12 & 0.55 \\

Baseline + L2P + LwF & 93.28 & 41.77 & 2.58 & 2.88 &  91.69 & 95.38 & \textbf{0.57} &  0.68\\
Baseline + DualPrompt + LwF & 92.74 & 42.15 & 2.67 & 2.21 & 91.47 & 95.63 &1.02 & 0.58 \\
% Baseline + L2P + LwF &  &  &  &  &  &  & &  \\
Baseline + L2P + $\text{DER}^\#$ & 92.65 & 42.55 & 2.68 & 2.17 & 91.47 & 95.43 & 0.34 & \textbf{0.13}  \\
% Baseline + DualPrompt + LwF &  &  &  &  &  &  & &  \\
Baseline + DualPrompt + $\text{DER}^\#$ & 92.91 & 41.93 & 2.83 & 3.20 & 91.01 & 95.22 & 1.23& 0.92 \\
% Baseline + startPrompt + LwF &  &  &  &  &  &  & &  \\
% Baseline + $\text{DER}^\#$  &  &  &  &  &  &  & &  \\
\midrule
\textbf{ONER} (Ours) & \textbf{94.53} & \textbf{49.66} & \textbf{0.91} & \textbf{1.33} & \textbf{93.36} & \textbf{97.26} & \underline{0.59} & \underline{0.15} \\
\bottomrule
\end{tabular}}
\caption{Comparison with different incremental learning methods on the MVTec AD dataset ($N=15$) after training on the last subset. Bold and underline highlight the best and second-best results. The symbol (\#) denotes methods that replay original samples from previous tasks.}
%methods that use task-specific models.
\label{tab:mvtec-prompt}
\end{table*}

\begin{table*}[!t]
\centering
{\footnotesize
\begin{tabular}{lcccccccc}
\toprule
\multirow{2}{*}{\textbf{Method}} & \multicolumn{4}{c}{\textbf{Pixel-level}} & \multicolumn{4}{c}{\textbf{Image-level}} \\
\cmidrule(lr){2-5} \cmidrule(lr){6-9}
& \multicolumn{2}{c}{\textbf{ACC} $\uparrow$} & \multicolumn{2}{c}{\textbf{FM} $\downarrow$} & \multicolumn{2}{c}{\textbf{ACC} $\uparrow$} & \multicolumn{2}{c}{\textbf{FM} $\downarrow$} \\
\cmidrule(lr){2-3} \cmidrule(lr){4-5} \cmidrule(lr){6-7} \cmidrule(lr){8-9}
& \textbf{AUROC} & \textbf{AUPR} & \textbf{AUROC} & \textbf{AUPR} & \textbf{AUROC} & \textbf{AUPR} & \textbf{AUROC} & \textbf{AUPR} \\
\midrule
% \multicolumn{5}{l}{\textit{Incremental Anomaly Detection Methods}} \\
Baseline + L2P  & 84.04 & 19.01 & 8.49 & 8.81 & \underline{78.89} & \underline{82.95} & \textbf{2.46} & \textbf{1.91} \\
Baseline + DualPrompt   & 86.43 & 19.73 & 6.13 & 8.54 & 76.56 & 80.64 & 5.48& 4.54\\
Baseline + L2P + LwF & 84.28 & 17.93 & 7.02 & 9.63 & 74.70 & 79.38 & 6.75 & 5.75 \\
Baseline + DualPrompt + LwF & 87.74 & 18.88 & 5.19 & 9.21 & 76.95 & 80.48 & 5.11& 4.57 \\

% Baseline + L2P + LwF &  &  &  &  &  &  & &  \\
Baseline + L2P + $\text{DER}^\#$ & 85.73 & 19.83 & 6.27 & 8.33 & 75.01 &  79.56 &  6.09 &  5.1\\
% Baseline + DualPrompt + LwF &  &  &  &  &  &  & &  \\
Baseline + DualPrompt + $\text{DER}^\#$ & \underline{88.84} & \underline{20.24} & \underline{2.71} & \underline{6.94} & 77.62 & 82.22 & 4.41 & 2.81 \\
% Baseline + startPrompt + LwF &  &  &  &  &  &  & &  \\

% Baseline + $\text{DER}^\#$  &  &  &  &  &  &  & &  \\
\midrule
\textbf{ONER} (Ours)& \textbf{90.58} & \textbf{27.87} & \textbf{2.39} & \textbf{1.82} & \textbf{83.14} & \textbf{86.61} & \underline{3.88} & \underline{2.70} \\
\bottomrule
\end{tabular}}
\caption{Comparison with different incremental learning methods on the VisA dataset ($N=12$) after training on the last subset. Bold and underline highlight the best and second-best results. The symbol (\#) denotes methods that replay original samples from previous tasks.}
%methods that use task-specific models.
\label{tab:visa-prompt}

\end{table*}
The second drawback of UCAD concerns testing efficiency and storage requirements. UCAD requires multiple comparisons—one for each task—to identify the task associated with the input image, followed by a final comparison to generate the result. In contrast, our method only requires a single comparison, enhancing its testing efficiency.
Regarding storage, UCAD needs to store task-specific features with a shape of $(2,196,1024)$, which includes both key and knowledge features for each new task. Our method, however, stores features with a shape of $(197,768)$, encompassing image-level prototypes (shape $(1,768)$)  and pixel-level prototypes (shape $(196,768)$), making our approach much more storage-efficient.

In summary, our method surpasses UCAD in several key areas: achieving higher accuracy with lower forgetting, enhanced stability, improved testing efficiency, and reduced storage requirements. By eliminating the need for task identification during inference, our approach avoids the cumulative errors inherent in UCAD, ensuring more reliable and stable results. Furthermore, our method optimizes testing efficiency by streamlining the process and minimizes storage demands, making it a more efficient and robust solution for incremental anomaly detection.

\section{Additional details}
\subsection{Details for evaluation metrics}
\textbf{Forgetting Measure (FM)} evaluates the model's resistance to catastrophic forgetting in a class-incremental setting. This metric assesses how well the model retains knowledge of previously learned tasks as new tasks are introduced. Lower FM values indicate better retention of prior knowledge and thus more stable learning.

Since there are two modes during testing including the end-to-end and staged approach, the calculation of FM varies for each mode.

\begin{itemize}

\item \textbf{End-to-end}: In this mode, a unified model is utilized for all tasks, which faces the issue of catastrophic forgetting. Therefore, the FM for the end-to-end approach is calculated as follows:
  \begin{equation}
  FM_{e}=\frac{1}{N-1}\sum_{i=1}^{N-1}\max_{j\in\{1,~\dots,~N-1\}}(\text{M}_{j,i}-\text{M}_{N,i}) ,
  \end{equation}
  where \( N \) is the total number of tasks, \( \text{M}_{j,i} \) represents the evaluation metric for task \( i \) measured after learning task \( j \), and \( \text{M}_{N,i} \) is the evaluation metric for task \( i \) measured after learning all tasks.
  
\item \textbf{Staged Approach}: 
Unlike end-to-end mode, staged approach first identifies each task via a classifier and subsequently applies a task-specific model for anomaly detection.
However, the effectiveness of the staged approach is significantly dependent on the accuracy of task identification in the first stage.

To this end, the FM for the staged approach is calculated as:
  \begin{equation}
  FM_{s} = \frac{1}{N}\sum_{i=1}^{N}\left(\text{M}_{\text{known},i} - \text{M}_{\text{pred},i} \right),
  \end{equation}
  where \( \text{M}_{\text{known},i} \) is the evaluation metric assuming the true class of the input image is known, and \( \text{M}_{\text{pred},i} \) is the evaluation metric when the class of the input image is predicted before anomaly detection.
\end{itemize}

These FMs help us understand the robustness of our model in retaining previously learned information and adapting to new tasks, ensuring a comprehensive evaluation of performance in class-incremental learning scenarios.

\subsection{Details for incremental classifier}
 \textbf{Incremental Classifier-based}: This strategy involves training an incremental classifier and task-specific models. The classifier is based on DER \cite{buzzega2020dark} and manages new classes, similar to UCAD’s task identification stage. Each new task requires a separate model, and the class-incremental classifier maintains categorization. We use a pre-trained ResNet18 model with selective freezing of the backbone’s final layer and training of the fully connected (fc) layer, employing SGD with a learning rate of 0.0005, a batch size of 10, and 25 epochs. For each task, five samples and their logits are saved for future training. This method achieved 69.45\% accuracy on the MVTec AD dataset ($N=15$) and 80.53\% on the VisA dataset ($N=12$).
 % \begin{table}[t]
% \centering
% \small
% % {\footnotesize
% \begin{tabular}{lcc}
% \toprule
% Method & Learnable Parameters & Epochs \\
% \midrule
% DRAEM~\textcolor{gray}{\tiny [ICCV21]} & 97.42M & 300 \\
% % GLAD~\textcolor{gray}{\tiny [ECCV24]} & 859.52M  & 280\\
% BGAD~\textcolor{gray}{\tiny [CVPR23]} & 3.39M & 100 \\
% % STPM~\textcolor{gray}{\tiny [BMVC21]} & & \\
% % SimpleNet~\textcolor{gray}{\tiny [CVPR23]} & 3.94M & 160 \\
% % \midrule
% DRAEM-Replay & 97.42M & 300\\
% BGAD-Replay & 3.39M & 100\\
% DRAEM-CLS* & (97.42+8.40)M & 300+10\\
% BGAD-CLS* & (3.39+8.40)M & 100+10\\
% % \midrule
% \hline

% CAD~\textcolor{gray}{\tiny [ACM MM23]} & 85.21M & 50 \\
% IUF~\textcolor{gray}{\tiny [ECCV24]} & 9.11M & 200 \\
% UCAD*~\textcolor{gray}{\tiny [AAAI24]} & 0.021M & 25 \\

% % \midrule
% \hline
% \textbf{ONER} (Ours) & \textbf{0.019M} & \textbf{5} \\
% \bottomrule
% \end{tabular}
% \caption{Statistics of learnable parameters and training epochs per task for different methods on the MVTec AD dataset.}
% \label{tab:parameter_epochs_statistics}
% \end{table}
\section{Additional experiments}
\subsection{Additional qualitative study}
Fig.~\ref{fig3} illustrates the substantial performance decline caused by task identification inaccuracies within a two-stage approach, highlighting its unreliability.
In contrast, our method directly processes input images, resulting in more stable and dependable detection outcomes.
\subsection{Experiments with different prompt-tuning method}
We enhance our baseline with two prompt-tuning methods: Learning to Prompt~(L2P)~\cite{Wang_Zhang_Lee_Zhang_Sun_Ren_Su_Perot_Dy_Pfister_2022} and DualPrompt~\cite{wang2022dualprompt}. 
Additionally, we further optimize these configurations by introducing LwF~\cite{DBLP:conf/eccv/LiH16}.
%, resulting in versions of our baseline enhanced with L2P and LwF, and DualPrompt and LwF.
% We also optimize the prompt structure by integrating the latest Visual Fourier Prompt Tuning (VFPT)~\cite{zeng2024visual}, leading to two further configurations: one with L2P and VFPT, and the other with DualPrompt and VFPT.
Furthermore, We also extend these configurations by introducing Dark Experience Replay~(DER)~\cite{buzzega2020dark}, which rehearses 5 images per tasks.
%, resulting in versions of our baseline enhanced with L2P and DER, and DualPrompt and DER.
It is important to highlight that we use $\mathcal{L}_{\text{TSC}}$ as the core loss function for prompt optimization. As demonstrated in Tables~\ref{tab:mvtec-prompt} -~\ref{tab:visa-prompt}, our method outperforms other incremental learning approaches.
\subsection{Experiments with incremental orders}
In the main paper, we follow UCAD's approach by organizing the incremental learning sequence alphabetically by category. To further validate our method's robustness, we conduct additional experiments using a randomly shuffled incremental order. As shown in Tab.~\ref{tab:order-visa} - \ref{tab:order-mvtec}, our method maintains consistent performance regardless of the sequence, indicating the robustness of the method.

\begin{table}[h]
% \centering
{\footnotesize
\begin{tabular}{lcccc}
\toprule
\textbf{Incremental Order} & \multicolumn{2}{c}{\textbf{Image-level}} & \multicolumn{2}{c}{\textbf{Pixel-level}} \\
\cmidrule(lr){2-3} \cmidrule(lr){4-5}
 &   \textbf{AUROC} & \textbf{AUPR} & \textbf{AUROC} & \textbf{AUPR} \\
\midrule
Alphabetical (Asc) & 83.14 & 86.61 & 90.58 & 27.87 \\
\midrule
% Alphabetical (Desc) & 80.08 & 83.76 & 84.39 & 20.90 \\
% \midrule
Random Order 1 &  83.27 & 86.63 & 90.74 & 25.88 \\
\midrule
Random Order 2 &  82.94 & 86.08 & 90.29 & 27.52 \\
\midrule
Random Order 3 &  81.99 & 85.71 & 90.14 & 26.04 \\
\bottomrule
\end{tabular}}
\caption{Evaluation of performance metrics on the VisA dataset across various incremental orders for our method.}
\label{tab:order-visa}

\end{table}

\begin{table}[h]
% \centering
{\footnotesize
\begin{tabular}{lcccc}
\toprule
\textbf{Incremental Order} & \multicolumn{2}{c}{\textbf{Image-level}} & \multicolumn{2}{c}{\textbf{Pixel-level}} \\
\cmidrule(lr){2-3} \cmidrule(lr){4-5}
 &   \textbf{AUROC} & \textbf{AUPR} & \textbf{AUROC} & \textbf{AUPR} \\
\midrule
Alphabetical (Asc) & 93.36 & 97.26 & 94.53 & 49.66 \\
\midrule
Random Order 1 & 93.94 & 97.29 & 93.69 & 48.90 \\
\midrule
Random Order 2 &  93.30 & 97.10 & 94.43 & 49.05 \\
\midrule
% Random Order 2 &  93.25 & 96.83 & 93.91 & 48.42 \\
% \midrule
Random Order 3 &  93.10 & 96.82 & 94.77 & 48.82 \\

\bottomrule
\end{tabular}}
\caption{Evaluation of performance metrics on the MVTec AD dataset across various incremental orders for our method.}
\label{tab:order-mvtec}

\end{table}

\end{appendices}
